# Supplementary material for: IISERB Brains at SemEval 2022 Task 6: A Deep-learning Framework to Identify Intended Sarcasm in English
Source: arXiv:2203.02244 source file (2022-03-04)
Supplement: Supplementary file 1 [file 60Appendix.tex]

\appendix

\section{Example Appendix}
\label{sec:appendix}

This is an appendix.
